# Supplementary material for: All-electron density functional calculations for electron and nuclear spin interactions in molecules and solids
Source: arXiv:1902.07377 ancillary file (2019-03-17)
Supplement: Supplementary file 1 [file SM.pdf]

# Supplemental Material for
# All-electron density functional calculations for electron and nuclear spin interactions in molecules and solids


Krishnendu Ghosh[1], He Ma[2,3], Vikram Gavini[1,4], and Giulia Galli[2,3,5]

[1]*Department of Mechanical Engineering, University of Michigan, Ann Arbor MI 48109*
[2]*The Institute for Molecular Engineering, University of Chicago, Chicago IL 60637*
[3]*Department of Chemistry, University of Chicago, Chicago IL 60637*
[4]*Department of Materials Science and Engineering, University of Michigan, Ann Arbor MI 48109 and*
[5]*Materials Science Division, Argonne National Laboratory, Lemont IL 60439*



(Dated: March 17, 2019)

## I. REAL SPACE COMPUTATION OF D-TENSOR FOR CRYSTALLINE SOLIDS

Here, we describe the mathematical formulation behind translating Eq. 5 (Eq. 6) to Eq. 7 (Eq. 8) in the main article for crystalline solids. Eq. 5, in a periodic system, has the following the form given by

$$M_{ab}^{ij,D} = \int_{\Omega}\int_{\mathbb{R}^3} f(\mathbf{r})\frac{\partial^2 G(\mathbf{r},\mathbf{r}^{'})}{\partial r_a \partial r_b^{'}} h(\mathbf{r}^{'}) d\mathbf{r}^{'} d\mathbf{r}\,, \tag{1}$$

with $h(\mathbf{r}^{'}) = \phi_j(\mathbf{r}^{'})\phi_j^*(\mathbf{r}^{'})$ and $f(\mathbf{r}) = \phi_i(\mathbf{r})\phi_i^*(\mathbf{r})$. $\Omega$ is the volume representing the unit cell. Integrating by parts with respect to $\mathbf{r}$, we arrive at

$$M_{ab}^{ij,D} = -\int_{\Omega}\frac{\partial f(\mathbf{r})}{\partial r_a}\int_{\mathbb{R}^3}\frac{\partial G(\mathbf{r},\mathbf{r}^{'})}{\partial r_b^{'}} h(\mathbf{r}^{'}) d\mathbf{r}^{'} d\mathbf{r} + \oint_{S(\Omega)} f(\mathbf{r})\Big(\int_{\mathbb{R}^3}\frac{\partial G(\mathbf{r},\mathbf{r}^{'})}{\partial r_b^{'}} h(\mathbf{r}^{'}) d\mathbf{r}^{'}\Big) d(\hat{\mathbf{a}}.\mathbf{S})\,. \tag{2}$$

Now noting the fact that $\frac{\partial G(\mathbf{r},\mathbf{r}^{'})}{\partial r_b^{'}} = -\frac{\partial G(\mathbf{r},\mathbf{r}^{'})}{\partial r_b}$, we can rewrite the second term on the right hand side of Eq. 2 as

$$M_{ab,2}^{ij,D} = -\oint_{S(\Omega)} f(\mathbf{r})\frac{\partial}{\partial r_b}\Big(\int_{\mathbb{R}^3} G(\mathbf{r},\mathbf{r}^{'}) h(\mathbf{r}^{'}) d\mathbf{r}^{'}\Big) d(\hat{\mathbf{a}}.\mathbf{S})\,. \tag{3}$$

The term within the parenthesis (let us denote it as $\Phi(\mathbf{r})$) can be obtained from the solution of the PDE, $\nabla^2\Phi(\mathbf{r}) = -4\pi h(\mathbf{r})$, with periodic boundary conditions on the unit cell domain, provided $\int_{\Omega} h(\mathbf{r})d\mathbf{r} = 0$. However, this condition is not valid while computing the direct part of the D-tensor, as $\int_{\Omega} h(\mathbf{r})d\mathbf{r} = 1$. Thus, we rewrite Eq. 3 as the sum of two terms, given by

$$M_{ab,2}^{ij,D} = -\oint_{S(\Omega)} f(\mathbf{r})\frac{\partial}{\partial r_b}\left(\int_{\mathbb{R}^3} G(\mathbf{r},\mathbf{r}^{'})\Big(h(\mathbf{r}^{'}) - \frac{1}{\Omega}\Big) d\mathbf{r}^{'}\right) d(\hat{\mathbf{a}}.\mathbf{S}) - \frac{1}{\Omega}\oint_{S(\Omega)} f(\mathbf{r})\Big(\int_{\mathbb{R}^3}\frac{\partial G(\mathbf{r},\mathbf{r}^{'})}{\partial r_b} d\mathbf{r}^{'}\Big) d(\hat{\mathbf{a}}.\mathbf{S})\,. \tag{4}$$

Considering the second term on the right hand side of Eq. 4, it is straightforward to show that the integral within the parenthesis (over $\mathbb{R}^3$) vanishes. Further, noting that the convolution integral within the parenthesis (over $\mathbb{R}^3$) of the first term of Eq. 4 is the given by the solution of the Poisson equation, the resulting field is periodic on the unit cell. Thus, the surface integral in the first term of Eq. 4 vanishes owing to the periodicity of the functions. Thus, Eq. 2 can be rewritten as

$$M_{ab}^{ij,D} = -\int_{\Omega}\frac{\partial f(\mathbf{r})}{\partial r_a}\int_{\mathbb{R}^3}\frac{\partial G(\mathbf{r},\mathbf{r}^{'})}{\partial r_b^{'}} h(\mathbf{r}^{'}) d\mathbf{r}^{'} d\mathbf{r}\,, \tag{5}$$

which, again, through integration by parts can be written as

$$M_{ab}^{ij,D} = \int_{\Omega}\int_{\mathbb{R}^3}\frac{\partial f(\mathbf{r})}{\partial r_a} G(\mathbf{r},\mathbf{r}^{'})\frac{\partial h(\mathbf{r}^{'})}{\partial r_b^{'}} d\mathbf{r}^{'} d\mathbf{r}\,, \tag{6}$$

which is same as Eq. 7 of the main article. We note that the boundary term, resulting from integration by parts, in the above equation vanishes as $G(\mathbf{r},\mathbf{r}^{'}) \to 0$ as $\mathbf{r}^{'} \to \infty$.

The treatment of the exchange term is similar. In this case, we define $h(\mathbf{r}^{'}) = \phi_i(\mathbf{r}^{'})\phi_j^*(\mathbf{r}^{'})$, and $f(\mathbf{r}) = \phi_i(\mathbf{r})\phi_j^*(\mathbf{r})$, $\forall\ i \neq j$. Thus, the condition $\int_{\Omega} h(\mathbf{r})d\mathbf{r} = 0$ holds from the orthogonality of the Kohn-Sham wavefunctions, and one need not split Eq. 3 into two parts as above. The rest of the arguments are identical.

## II. CONVERGENCE TESTS FOR GTO CALCULATIONS WITH CC- BASIS SETS

In this section we present $A^{\rm iso}$, $A^{\rm dip}_{33}$, $D$ and $V_{33}$ (see main text) computed with GTO DFT as a function of basis sets: cc-pVDZ ($\zeta = 2$), cc-pVTZ ($\zeta = 3$), cc-pVQZ ($\zeta = 4$), cc-pV5Z ($\zeta = 5$). According to the following plots, in many cases spin Hamiltonian parameters do not converge with respect to basis in a reasonable manner. Therefore, it is challenging to extrapolate the results to the complete basis set (CBS) limit, as is usually done for the calculation of DFT total energies.

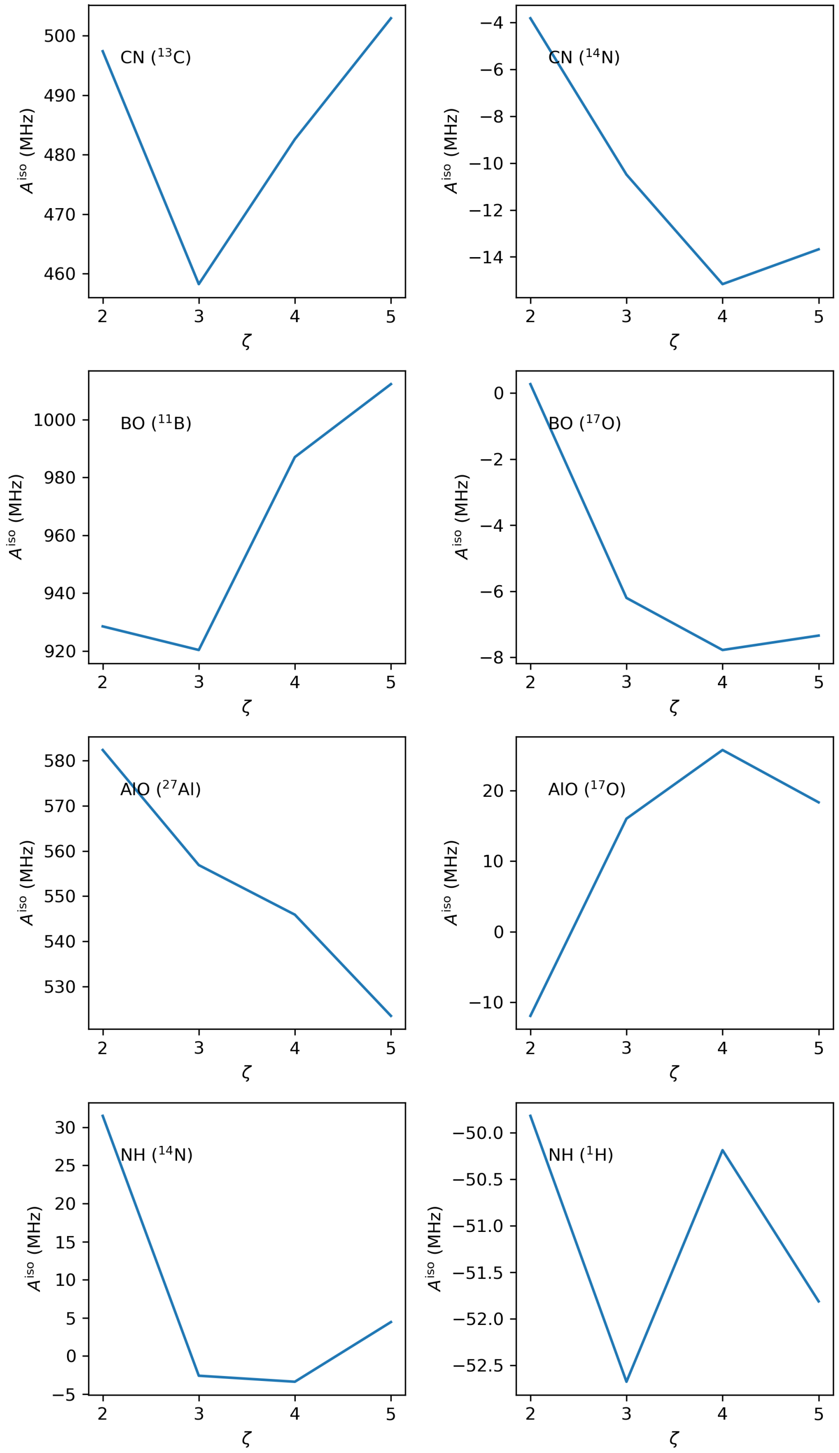


Figure 1. $A^{\rm iso}$ as a function of basis set.

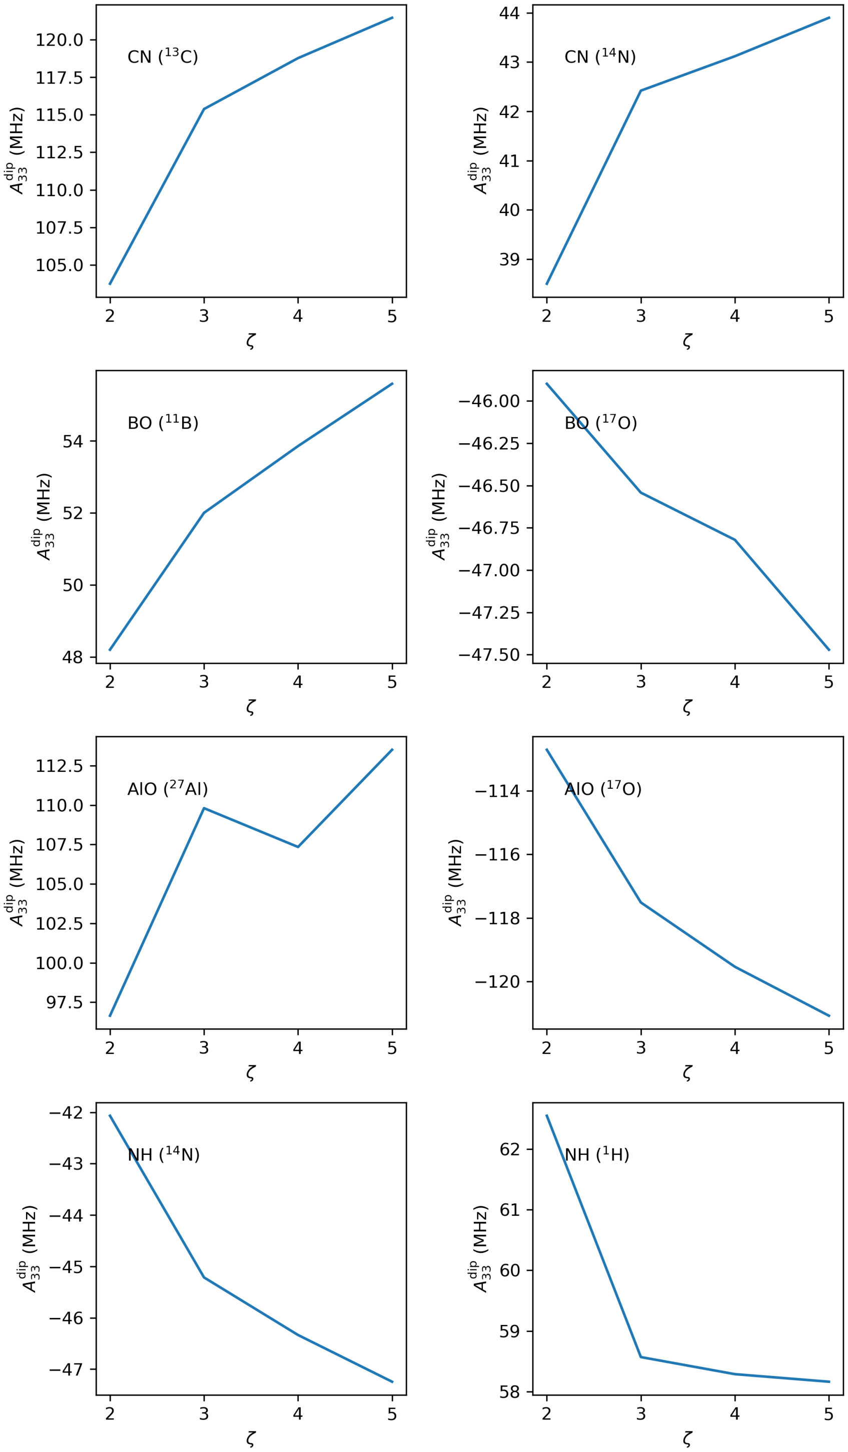


Figure 2. $A_{33}^{\rm dip}$ as a function of basis set.

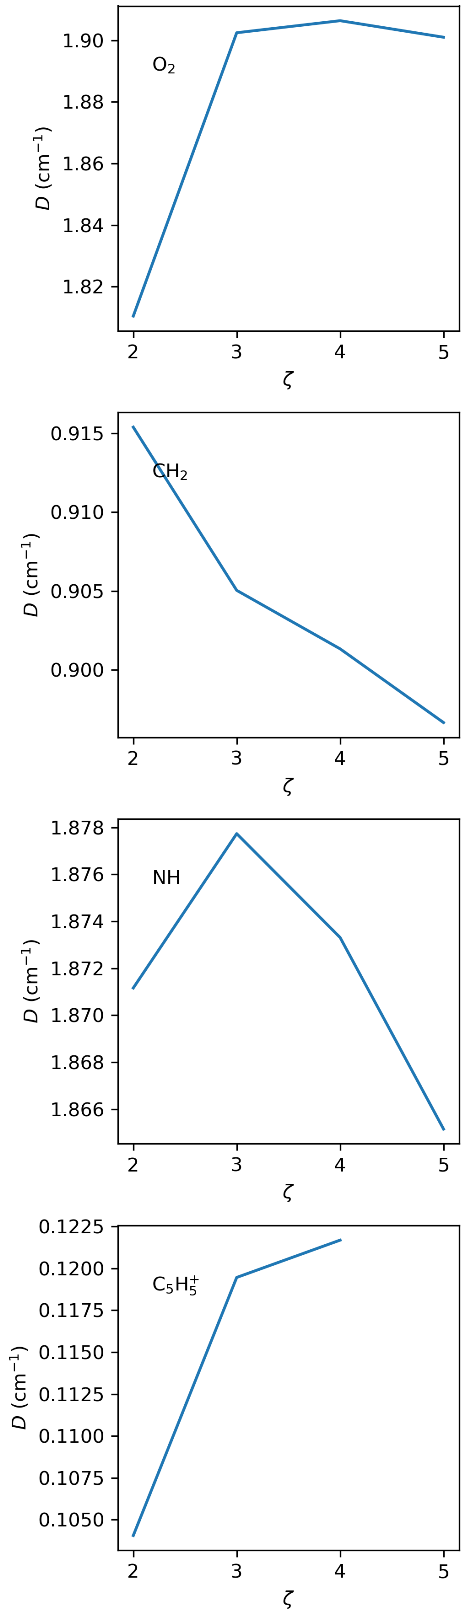


Figure 3. $D$ as a function of basis set. cc-pV5Z calculation for $C_5H_5^+$ is not performed due to computational cost.

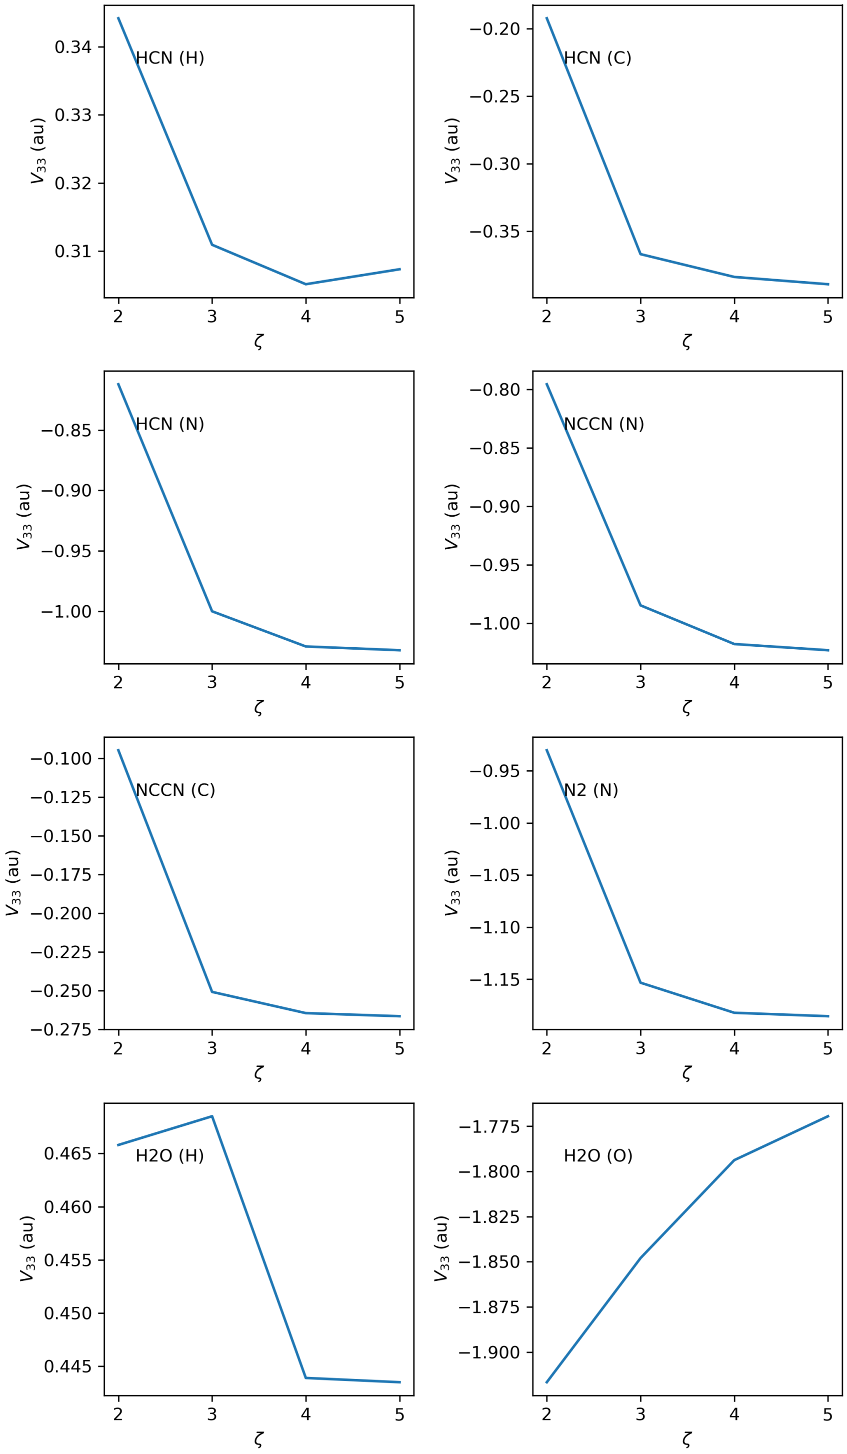


Figure 4. $V_{33}$ as a function of basis set.
